# Supplementary material for: Two by Two: Learning Multi-Task Pairwise Objects Assembly for Generalizable Robot Manipulation
Source: arXiv:2504.06961 source file (2026-08-15)
Supplement: Supplementary file 1 [file _supplementary.tex]

\input{_constants}
\review % \review OR \cameraready

\documentclass[10pt,twocolumn,letterpaper]{article}
\input{cvpr_header}
\myexternaldocument{_main}

\usepackage{amsmath} 
\usepackage{amssymb}

\begin{document}

%% TITLE
\title{Two by Two \includegraphics[height=0.04\linewidth]{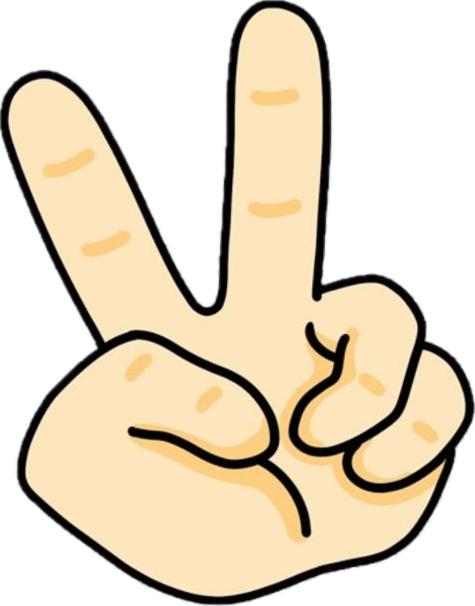}: Learning Cross-Task Pairwise Objects Assembly \\ for Generalizable Robot Manipulation}
\author{\authorBlock}
\maketitlesupplementary
%%

%% TITLE
\title{Two by Two \includegraphics[height=0.04\linewidth]{figs/icon.png}: Learning Cross-Task Pairwise Objects Assembly \\ for Generalizable Robot Manipulation}
\author{\authorBlock}
\maketitlesupplementary

\input{12_appendix}

\clearpage
\clearpage

{\small
\bibliographystyle{ieeenat_fullname}
\bibliography{11_references}
}

\input{12_appendix}

\clearpage
\clearpage

{\small
\bibliographystyle{ieeenat_fullname}
\bibliography{11_references}
}

\end{document}
